# Supplementary material for: MagicStick: Controllable Video Editing via Control Handle Transformations
Source: arXiv:2312.03047 source file (2024-11-18)
Supplement: Supplementary file 1 [file X_supp.tex]

\clearpage
\setcounter{page}{1}
% \documentclass[onecolumn]{article}
% \maketitlesupplementary

The supplementary material is organized as follows. In Sec.~\ref{sec:Implementation Details}, we provide the implementation details for controllable video editing.
Then, the demo video is presented in Sec.~\ref{sec:video}.

\appendix
\section{Implementation Details}
\label{sec:Implementation Details}

We implement our method based on the pre-trained Stable Diffusion (SD)~\cite{rombach2022high} and ControlNet~\cite{zhang2023adding} at 100 iterations. We sample 8 uniform frames at the resolution of $512\times512$ from the input video and ﬁne-tune the models for about 5 minutes on a single 24G NVIDIA RTX 3090Ti GPU. The time cost of training stage is cheap.
The learning rate is $3 \times 10^{-5} $.
During editing, the attentions are fused only in the DDIM step at $t\in [0.5 \times  T, T]$ with total timesteps $T = 50$. We adopt DDIM sampler~\cite{song2020denoising} with classiﬁer-free guidance~\cite{ho2022classifier}
in our experiments. The source text prompt of the input video is generated via the image caption model~\cite{li2022blip} and then replaced or modified some words manually according to different editing needs. There are mainly two hyperparameters in our proposed designs: a) Timestep of the self-attention blending, following FateZero~\cite{qi2023fatezero}, smaller timestep allows for more self-attention from the inversion process, thereby preserving the structure and motion more effectively. b) Threshold for the blending mask, smaller threshold utilizes more self-attention maps from the editing process, thereby enhancing the results of editing.

\section{Demo Video}
% \label{sec:video}
% We provide a demo video in mp4 format to present more details.
% \vspace{-1.5em}
% \paragraph{Overview.} In this part, we show the pipeline of controllable video editing via modifying the controlling conditions. The bird in the source video can be resized to various sizes through control signal editing.
% \vspace{-1.5em}
% \paragraph{Video Results.} We provide more results on size editing, position editing, appearance editing, and human motion editing to validate the effectiveness of the proposed method.
% \vspace{-2.6em}
% \paragraph{Method Animation.} We provide an animation of our method for a better understanding.
% \vspace{-1.5em}
% \paragraph{Baseline Comparisons.} We demonstrate comparisons with previous methods qualitatively in the video.
% \vspace{-1.5em}
% \paragraph{More Applications.} In our paper, we have shown our powerful ability in video property editing (\textit{e.g.,} shape, size, location, motion). In the demo video, we further present some promising applications of the proposed method, including 
% (1) controllable object replication: our method achieves the replication of the object and its related motion to different positions in the video.
% (2) controllable object removal: object removal by removing the word of the target object in the source prompt and the control signal in the first condition frame.
% (3) controllable object motion: Given a motion and initial image, our method is capable of guiding an object along a specified path.

\noindent\textbf{Object motion control.} An interesting application of our method is to edit the motion of objects, which can be achieved by modifying the control signal frames. As shown in Fig.~\ref{fig:motion_show}, We have the capability to create a consistent video clip while following the given motion of the synthesized \enquote{\texttt{balloon}}, ensuring the consistency of the background at the same time. 

\begin{figure*}
    \centering
    \includegraphics[width=\linewidth]{images/object_motion.pdf}
    \caption{\textit{\textbf{Object motion control.}} We present an interesting application using our method. Given an image and motion of the object, we can generate a consistent video clip and precisely control the synthesized object motions. Zoom in for the best view.
    }
    \label{fig:motion_show}
\end{figure*}
